# Supplementary material for: A geometric reformulation of the bilevel parameter optimization problem to a single level non-linear programming problem with applications to phase equilibria
Source: arXiv:2608.17806 source file (2026-08-18)
Supplement: Supplementary file 2 [file appendix-refrig-ternary_figure_blocks.tex]

% Auto-generated by figures/appendix-refrig-ternary/plot.py.
% One figure environment per Kato & Nishiumi (2006) tie-line.

\begin{figure}[ht]
\centering
\begin{minipage}[t]{0.48\textwidth}
  \centering
  \includegraphics[width=\linewidth]{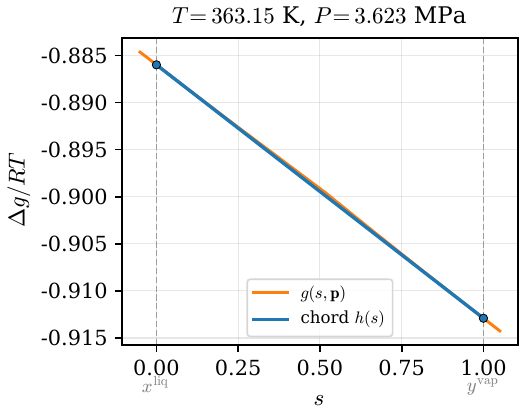}
\end{minipage}
\hfill
\begin{minipage}[t]{0.48\textwidth}
  \centering
  \includegraphics[width=\linewidth]{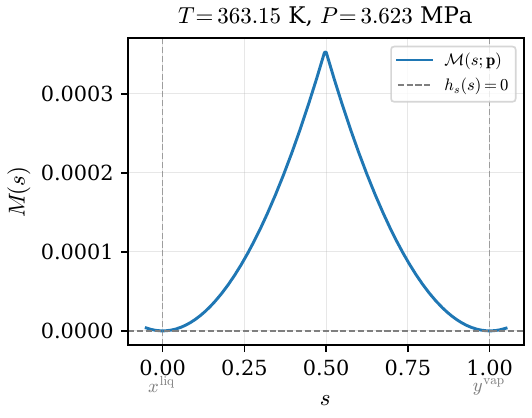}
\end{minipage}
\caption{Tie line 1 of the Kato--Nishiumi R-407C ternary set at $T = 363.15$~K, $P = 3.623$~MPa. Left: reduced Gibbs energy $g$ along the model tie-line section with the common-tangent chord $h$; right: dual manifold $\mathcal{M} = g - h$.}
\label{fig:appendix-refrig-tie01}
\end{figure}

\begin{figure}[ht]
\centering
\begin{minipage}[t]{0.48\textwidth}
  \centering
  \includegraphics[width=\linewidth]{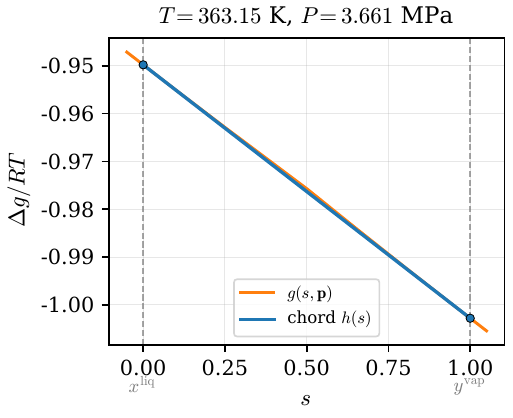}
\end{minipage}
\hfill
\begin{minipage}[t]{0.48\textwidth}
  \centering
  \includegraphics[width=\linewidth]{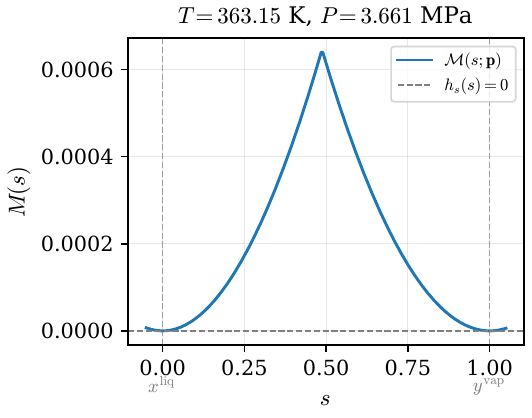}
\end{minipage}
\caption{Tie line 2 of the Kato--Nishiumi R-407C ternary set at $T = 363.15$~K, $P = 3.661$~MPa. Left: reduced Gibbs energy $g$ along the model tie-line section with the common-tangent chord $h$; right: dual manifold $\mathcal{M} = g - h$.}
\label{fig:appendix-refrig-tie02}
\end{figure}

\begin{figure}[ht]
\centering
\begin{minipage}[t]{0.48\textwidth}
  \centering
  \includegraphics[width=\linewidth]{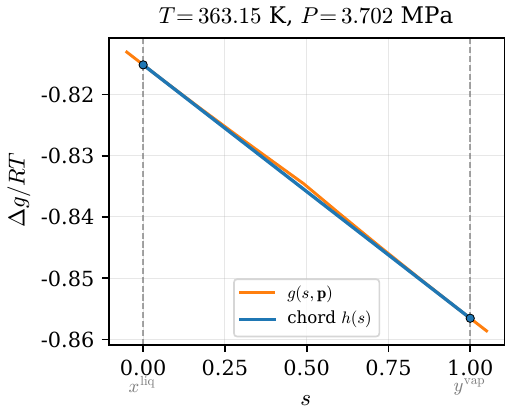}
\end{minipage}
\hfill
\begin{minipage}[t]{0.48\textwidth}
  \centering
  \includegraphics[width=\linewidth]{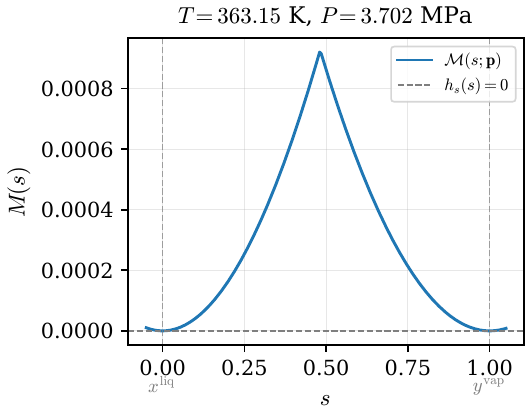}
\end{minipage}
\caption{Tie line 3 of the Kato--Nishiumi R-407C ternary set at $T = 363.15$~K, $P = 3.702$~MPa. Left: reduced Gibbs energy $g$ along the model tie-line section with the common-tangent chord $h$; right: dual manifold $\mathcal{M} = g - h$.}
\label{fig:appendix-refrig-tie03}
\end{figure}

\begin{figure}[ht]
\centering
\begin{minipage}[t]{0.48\textwidth}
  \centering
  \includegraphics[width=\linewidth]{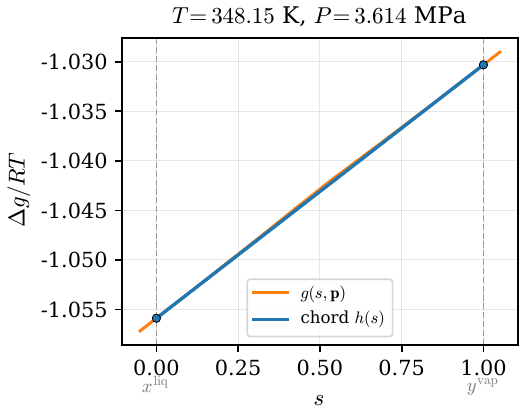}
\end{minipage}
\hfill
\begin{minipage}[t]{0.48\textwidth}
  \centering
  \includegraphics[width=\linewidth]{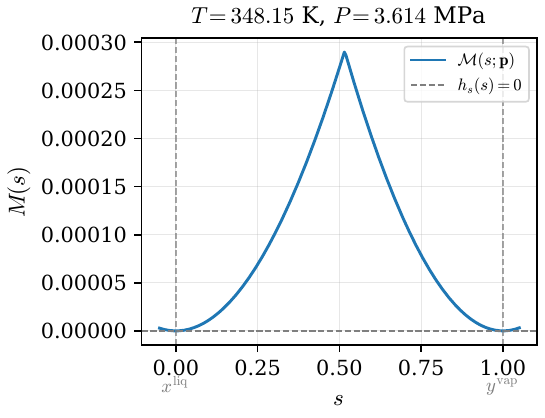}
\end{minipage}
\caption{Tie line 4 of the Kato--Nishiumi R-407C ternary set at $T = 348.15$~K, $P = 3.614$~MPa. Left: reduced Gibbs energy $g$ along the model tie-line section with the common-tangent chord $h$; right: dual manifold $\mathcal{M} = g - h$.}
\label{fig:appendix-refrig-tie04}
\end{figure}

\begin{figure}[ht]
\centering
\begin{minipage}[t]{0.48\textwidth}
  \centering
  \includegraphics[width=\linewidth]{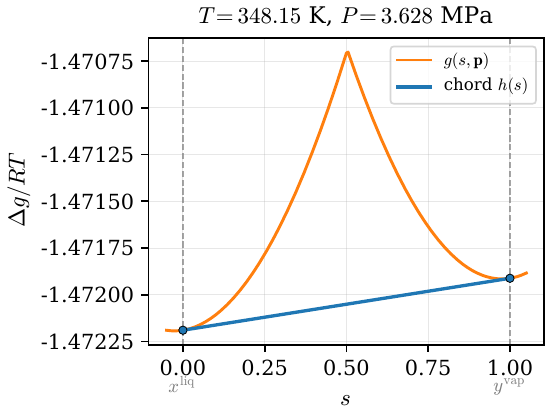}
\end{minipage}
\hfill
\begin{minipage}[t]{0.48\textwidth}
  \centering
  \includegraphics[width=\linewidth]{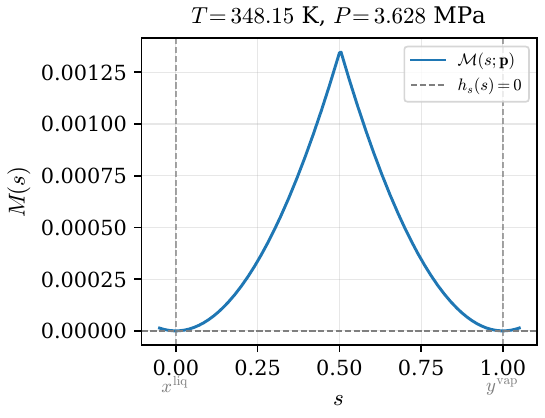}
\end{minipage}
\caption{Tie line 5 of the Kato--Nishiumi R-407C ternary set at $T = 348.15$~K, $P = 3.628$~MPa. Left: reduced Gibbs energy $g$ along the model tie-line section with the common-tangent chord $h$; right: dual manifold $\mathcal{M} = g - h$.}
\label{fig:appendix-refrig-tie05}
\end{figure}

\begin{figure}[ht]
\centering
\begin{minipage}[t]{0.48\textwidth}
  \centering
  \includegraphics[width=\linewidth]{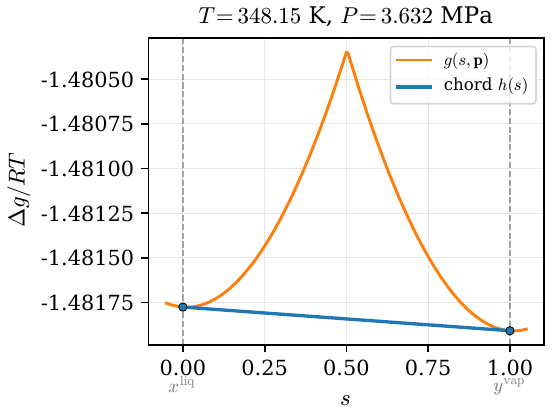}
\end{minipage}
\hfill
\begin{minipage}[t]{0.48\textwidth}
  \centering
  \includegraphics[width=\linewidth]{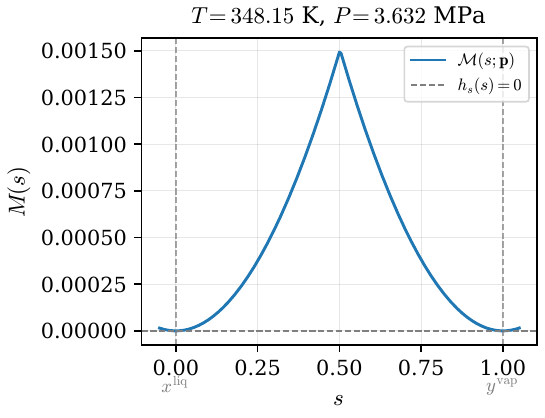}
\end{minipage}
\caption{Tie line 6 of the Kato--Nishiumi R-407C ternary set at $T = 348.15$~K, $P = 3.632$~MPa. Left: reduced Gibbs energy $g$ along the model tie-line section with the common-tangent chord $h$; right: dual manifold $\mathcal{M} = g - h$.}
\label{fig:appendix-refrig-tie06}
\end{figure}

\begin{figure}[ht]
\centering
\begin{minipage}[t]{0.48\textwidth}
  \centering
  \includegraphics[width=\linewidth]{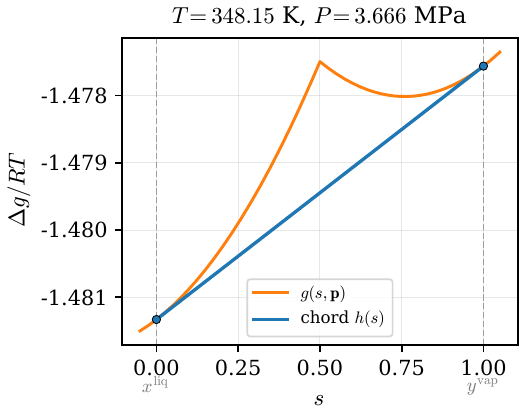}
\end{minipage}
\hfill
\begin{minipage}[t]{0.48\textwidth}
  \centering
  \includegraphics[width=\linewidth]{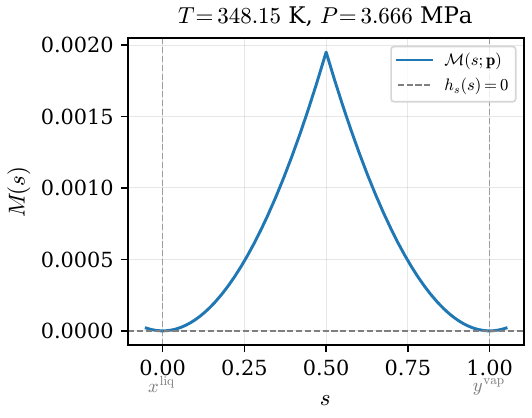}
\end{minipage}
\caption{Tie line 7 of the Kato--Nishiumi R-407C ternary set at $T = 348.15$~K, $P = 3.666$~MPa. Left: reduced Gibbs energy $g$ along the model tie-line section with the common-tangent chord $h$; right: dual manifold $\mathcal{M} = g - h$.}
\label{fig:appendix-refrig-tie07}
\end{figure}

\begin{figure}[ht]
\centering
\begin{minipage}[t]{0.48\textwidth}
  \centering
  \includegraphics[width=\linewidth]{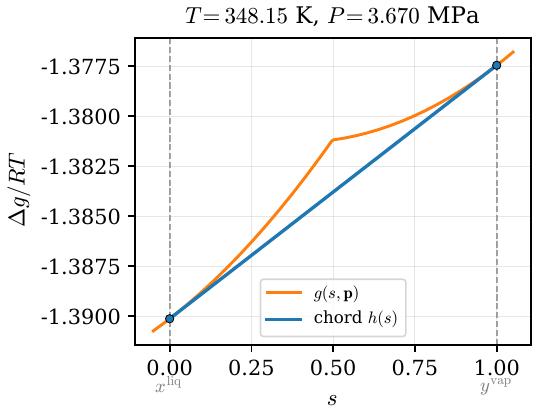}
\end{minipage}
\hfill
\begin{minipage}[t]{0.48\textwidth}
  \centering
  \includegraphics[width=\linewidth]{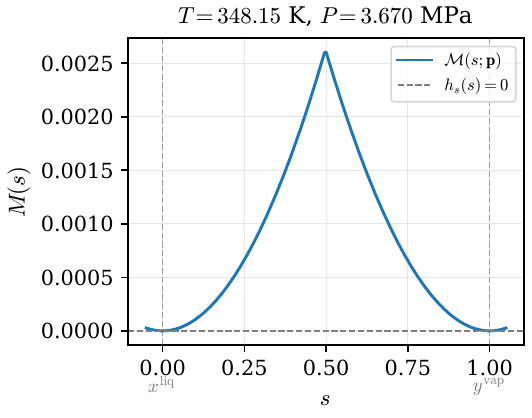}
\end{minipage}
\caption{Tie line 8 of the Kato--Nishiumi R-407C ternary set at $T = 348.15$~K, $P = 3.670$~MPa. Left: reduced Gibbs energy $g$ along the model tie-line section with the common-tangent chord $h$; right: dual manifold $\mathcal{M} = g - h$.}
\label{fig:appendix-refrig-tie08}
\end{figure}

\begin{figure}[ht]
\centering
\begin{minipage}[t]{0.48\textwidth}
  \centering
  \includegraphics[width=\linewidth]{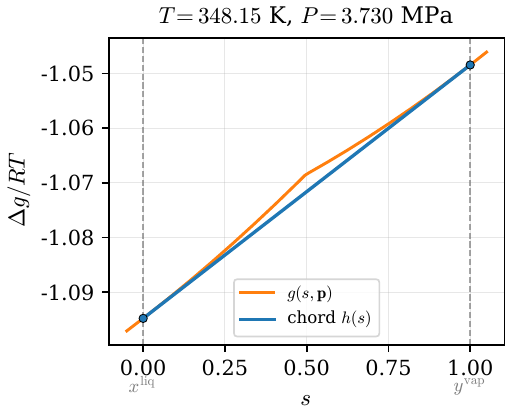}
\end{minipage}
\hfill
\begin{minipage}[t]{0.48\textwidth}
  \centering
  \includegraphics[width=\linewidth]{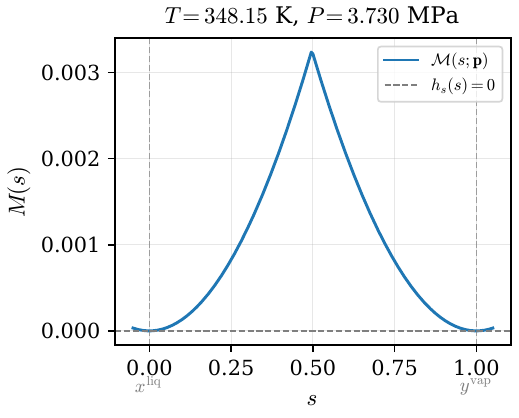}
\end{minipage}
\caption{Tie line 9 of the Kato--Nishiumi R-407C ternary set at $T = 348.15$~K, $P = 3.730$~MPa. Left: reduced Gibbs energy $g$ along the model tie-line section with the common-tangent chord $h$; right: dual manifold $\mathcal{M} = g - h$.}
\label{fig:appendix-refrig-tie09}
\end{figure}

\begin{figure}[ht]
\centering
\begin{minipage}[t]{0.48\textwidth}
  \centering
  \includegraphics[width=\linewidth]{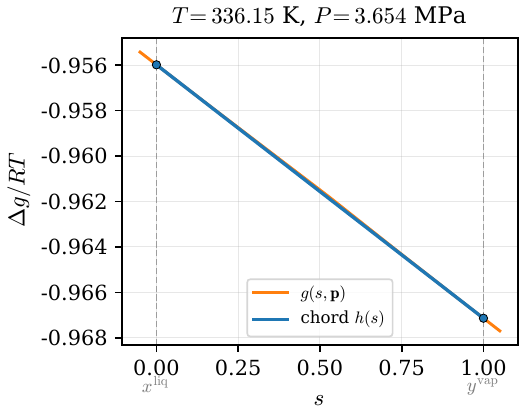}
\end{minipage}
\hfill
\begin{minipage}[t]{0.48\textwidth}
  \centering
  \includegraphics[width=\linewidth]{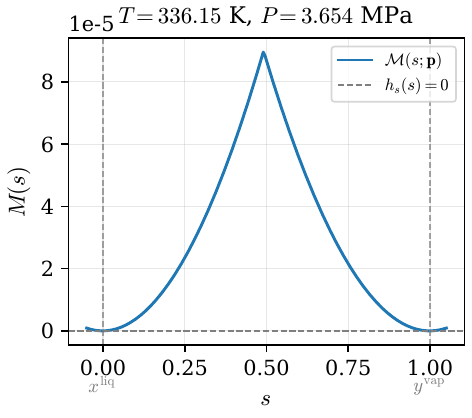}
\end{minipage}
\caption{Tie line 10 of the Kato--Nishiumi R-407C ternary set at $T = 336.15$~K, $P = 3.654$~MPa. Left: reduced Gibbs energy $g$ along the model tie-line section with the common-tangent chord $h$; right: dual manifold $\mathcal{M} = g - h$.}
\label{fig:appendix-refrig-tie10}
\end{figure}

\begin{figure}[ht]
\centering
\begin{minipage}[t]{0.48\textwidth}
  \centering
  \includegraphics[width=\linewidth]{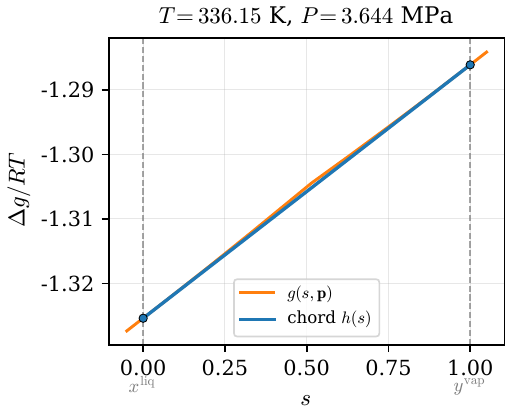}
\end{minipage}
\hfill
\begin{minipage}[t]{0.48\textwidth}
  \centering
  \includegraphics[width=\linewidth]{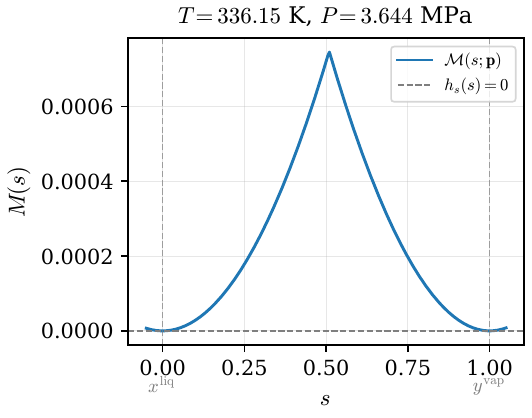}
\end{minipage}
\caption{Tie line 11 of the Kato--Nishiumi R-407C ternary set at $T = 336.15$~K, $P = 3.644$~MPa. Left: reduced Gibbs energy $g$ along the model tie-line section with the common-tangent chord $h$; right: dual manifold $\mathcal{M} = g - h$.}
\label{fig:appendix-refrig-tie11}
\end{figure}

\begin{figure}[ht]
\centering
\begin{minipage}[t]{0.48\textwidth}
  \centering
  \includegraphics[width=\linewidth]{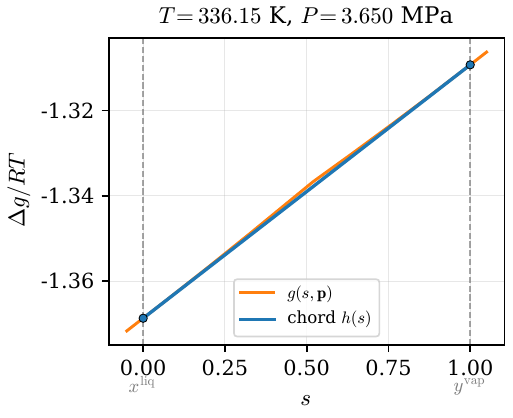}
\end{minipage}
\hfill
\begin{minipage}[t]{0.48\textwidth}
  \centering
  \includegraphics[width=\linewidth]{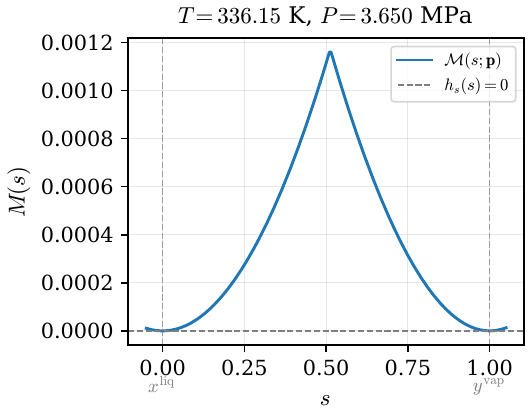}
\end{minipage}
\caption{Tie line 12 of the Kato--Nishiumi R-407C ternary set at $T = 336.15$~K, $P = 3.650$~MPa. Left: reduced Gibbs energy $g$ along the model tie-line section with the common-tangent chord $h$; right: dual manifold $\mathcal{M} = g - h$.}
\label{fig:appendix-refrig-tie12}
\end{figure}

\begin{figure}[ht]
\centering
\begin{minipage}[t]{0.48\textwidth}
  \centering
  \includegraphics[width=\linewidth]{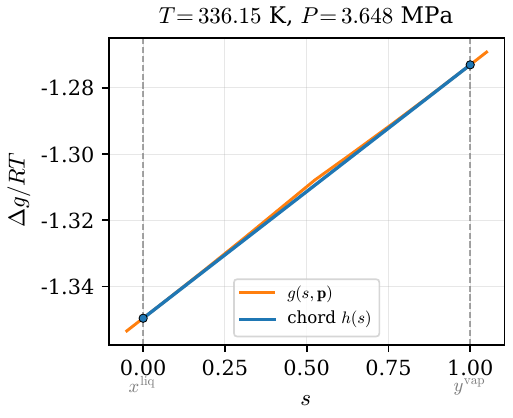}
\end{minipage}
\hfill
\begin{minipage}[t]{0.48\textwidth}
  \centering
  \includegraphics[width=\linewidth]{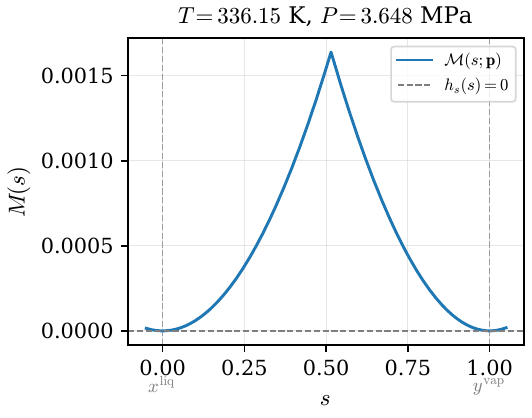}
\end{minipage}
\caption{Tie line 13 of the Kato--Nishiumi R-407C ternary set at $T = 336.15$~K, $P = 3.648$~MPa. Left: reduced Gibbs energy $g$ along the model tie-line section with the common-tangent chord $h$; right: dual manifold $\mathcal{M} = g - h$.}
\label{fig:appendix-refrig-tie13}
\end{figure}

\begin{figure}[ht]
\centering
\begin{minipage}[t]{0.48\textwidth}
  \centering
  \includegraphics[width=\linewidth]{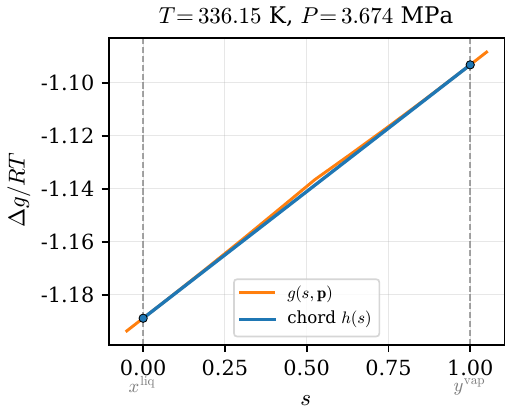}
\end{minipage}
\hfill
\begin{minipage}[t]{0.48\textwidth}
  \centering
  \includegraphics[width=\linewidth]{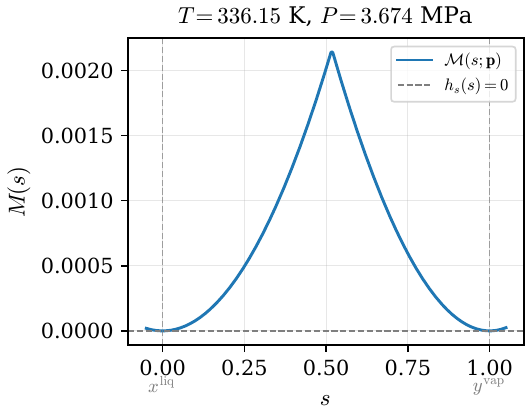}
\end{minipage}
\caption{Tie line 14 of the Kato--Nishiumi R-407C ternary set at $T = 336.15$~K, $P = 3.674$~MPa. Left: reduced Gibbs energy $g$ along the model tie-line section with the common-tangent chord $h$; right: dual manifold $\mathcal{M} = g - h$.}
\label{fig:appendix-refrig-tie14}
\end{figure}

\begin{figure}[ht]
\centering
\begin{minipage}[t]{0.48\textwidth}
  \centering
  \includegraphics[width=\linewidth]{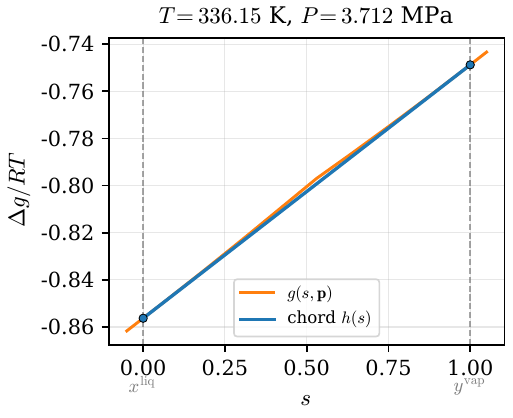}
\end{minipage}
\hfill
\begin{minipage}[t]{0.48\textwidth}
  \centering
  \includegraphics[width=\linewidth]{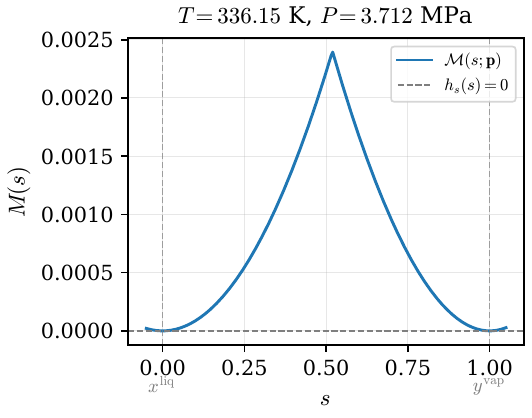}
\end{minipage}
\caption{Tie line 15 of the Kato--Nishiumi R-407C ternary set at $T = 336.15$~K, $P = 3.712$~MPa. Left: reduced Gibbs energy $g$ along the model tie-line section with the common-tangent chord $h$; right: dual manifold $\mathcal{M} = g - h$.}
\label{fig:appendix-refrig-tie15}
\end{figure}

\begin{figure}[ht]
\centering
\begin{minipage}[t]{0.48\textwidth}
  \centering
  \includegraphics[width=\linewidth]{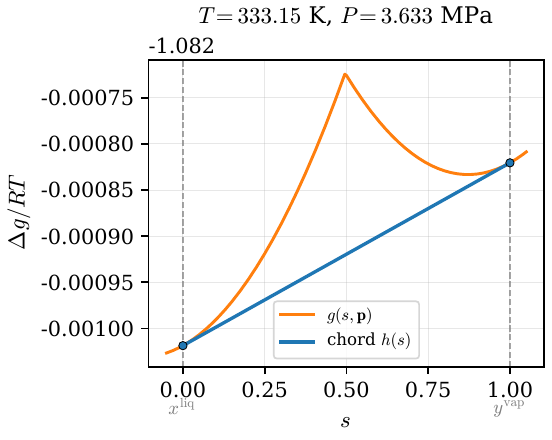}
\end{minipage}
\hfill
\begin{minipage}[t]{0.48\textwidth}
  \centering
  \includegraphics[width=\linewidth]{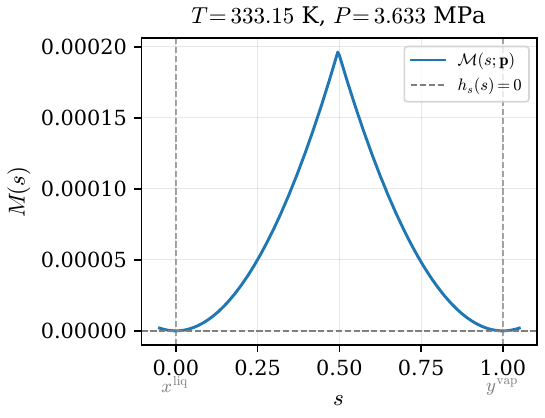}
\end{minipage}
\caption{Tie line 16 of the Kato--Nishiumi R-407C ternary set at $T = 333.15$~K, $P = 3.633$~MPa. Left: reduced Gibbs energy $g$ along the model tie-line section with the common-tangent chord $h$; right: dual manifold $\mathcal{M} = g - h$.}
\label{fig:appendix-refrig-tie16}
\end{figure}

\begin{figure}[ht]
\centering
\begin{minipage}[t]{0.48\textwidth}
  \centering
  \includegraphics[width=\linewidth]{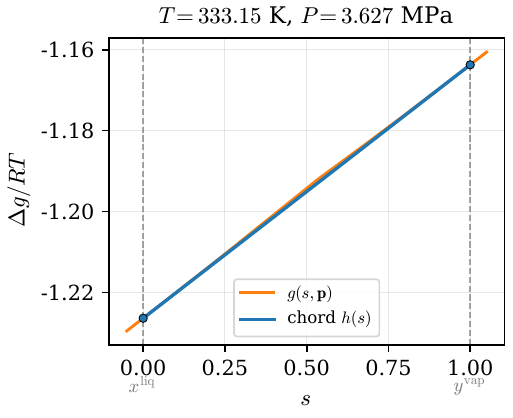}
\end{minipage}
\hfill
\begin{minipage}[t]{0.48\textwidth}
  \centering
  \includegraphics[width=\linewidth]{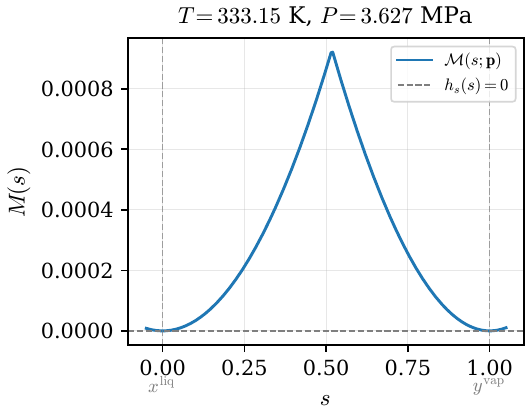}
\end{minipage}
\caption{Tie line 17 of the Kato--Nishiumi R-407C ternary set at $T = 333.15$~K, $P = 3.627$~MPa. Left: reduced Gibbs energy $g$ along the model tie-line section with the common-tangent chord $h$; right: dual manifold $\mathcal{M} = g - h$.}
\label{fig:appendix-refrig-tie17}
\end{figure}

\begin{figure}[ht]
\centering
\begin{minipage}[t]{0.48\textwidth}
  \centering
  \includegraphics[width=\linewidth]{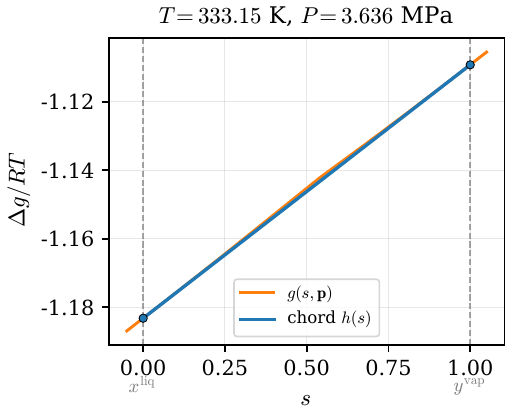}
\end{minipage}
\hfill
\begin{minipage}[t]{0.48\textwidth}
  \centering
  \includegraphics[width=\linewidth]{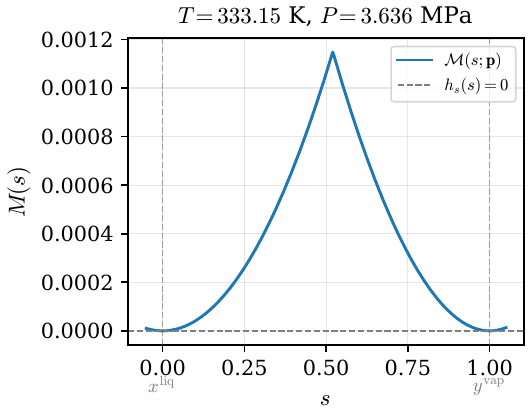}
\end{minipage}
\caption{Tie line 18 of the Kato--Nishiumi R-407C ternary set at $T = 333.15$~K, $P = 3.636$~MPa. Left: reduced Gibbs energy $g$ along the model tie-line section with the common-tangent chord $h$; right: dual manifold $\mathcal{M} = g - h$.}
\label{fig:appendix-refrig-tie18}
\end{figure}

\begin{figure}[ht]
\centering
\begin{minipage}[t]{0.48\textwidth}
  \centering
  \includegraphics[width=\linewidth]{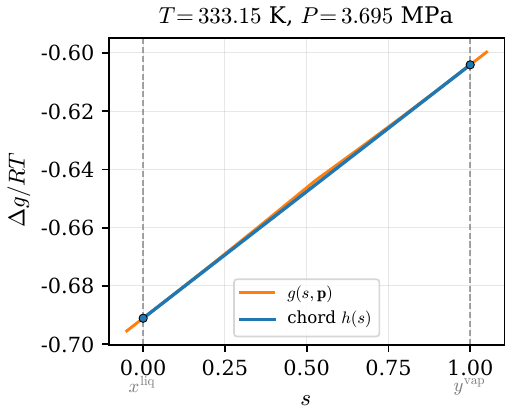}
\end{minipage}
\hfill
\begin{minipage}[t]{0.48\textwidth}
  \centering
  \includegraphics[width=\linewidth]{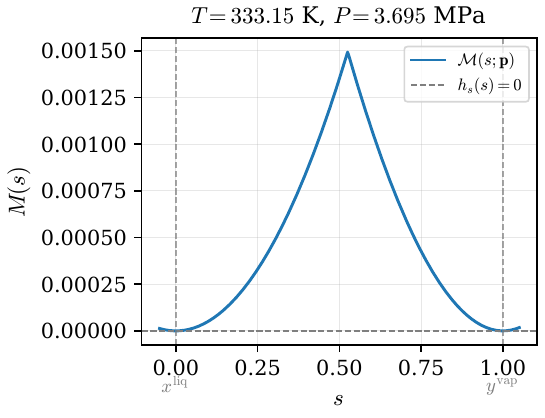}
\end{minipage}
\caption{Tie line 19 of the Kato--Nishiumi R-407C ternary set at $T = 333.15$~K, $P = 3.695$~MPa. Left: reduced Gibbs energy $g$ along the model tie-line section with the common-tangent chord $h$; right: dual manifold $\mathcal{M} = g - h$.}
\label{fig:appendix-refrig-tie19}
\end{figure}

\begin{figure}[ht]
\centering
\begin{minipage}[t]{0.48\textwidth}
  \centering
  \includegraphics[width=\linewidth]{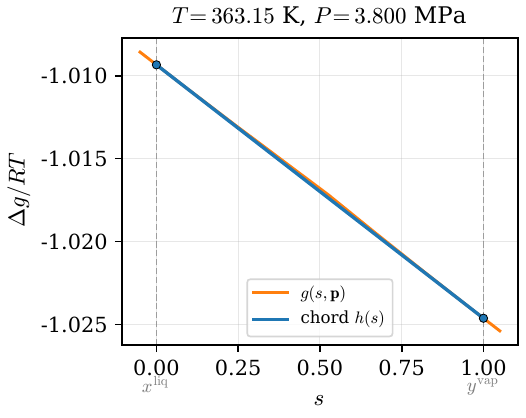}
\end{minipage}
\hfill
\begin{minipage}[t]{0.48\textwidth}
  \centering
  \includegraphics[width=\linewidth]{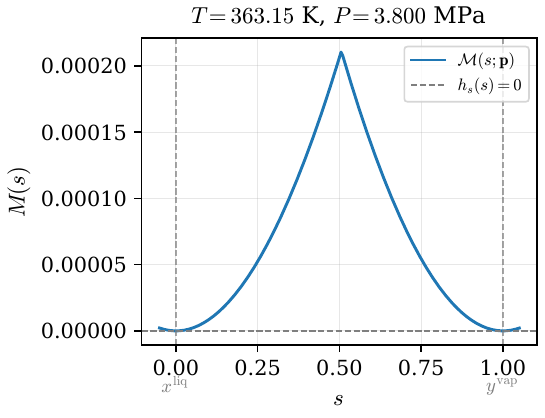}
\end{minipage}
\caption{Tie line 20 of the Kato--Nishiumi R-407C ternary set at $T = 363.15$~K, $P = 3.800$~MPa. Left: reduced Gibbs energy $g$ along the model tie-line section with the common-tangent chord $h$; right: dual manifold $\mathcal{M} = g - h$.}
\label{fig:appendix-refrig-tie20}
\end{figure}

\begin{figure}[ht]
\centering
\begin{minipage}[t]{0.48\textwidth}
  \centering
  \includegraphics[width=\linewidth]{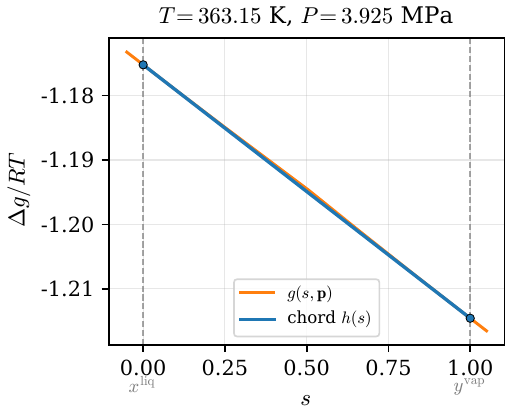}
\end{minipage}
\hfill
\begin{minipage}[t]{0.48\textwidth}
  \centering
  \includegraphics[width=\linewidth]{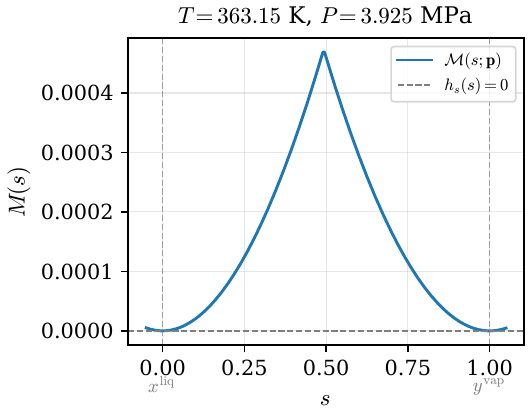}
\end{minipage}
\caption{Tie line 21 of the Kato--Nishiumi R-407C ternary set at $T = 363.15$~K, $P = 3.925$~MPa. Left: reduced Gibbs energy $g$ along the model tie-line section with the common-tangent chord $h$; right: dual manifold $\mathcal{M} = g - h$.}
\label{fig:appendix-refrig-tie21}
\end{figure}

\begin{figure}[ht]
\centering
\begin{minipage}[t]{0.48\textwidth}
  \centering
  \includegraphics[width=\linewidth]{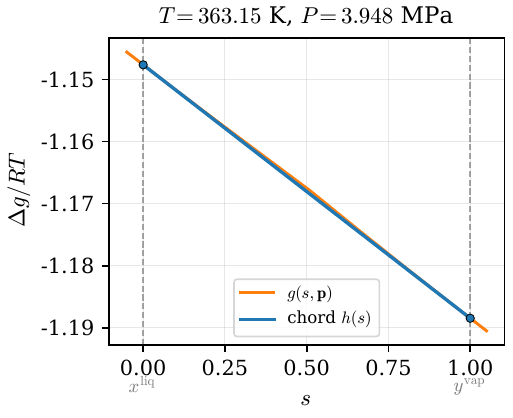}
\end{minipage}
\hfill
\begin{minipage}[t]{0.48\textwidth}
  \centering
  \includegraphics[width=\linewidth]{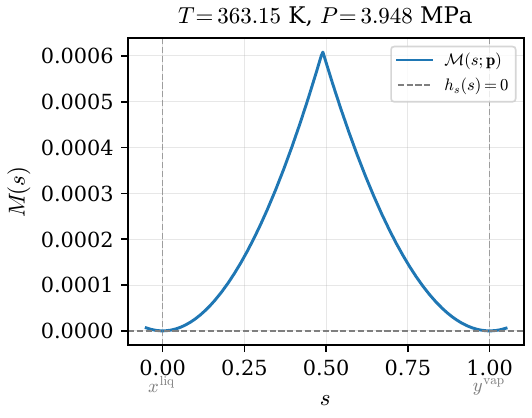}
\end{minipage}
\caption{Tie line 22 of the Kato--Nishiumi R-407C ternary set at $T = 363.15$~K, $P = 3.948$~MPa. Left: reduced Gibbs energy $g$ along the model tie-line section with the common-tangent chord $h$; right: dual manifold $\mathcal{M} = g - h$.}
\label{fig:appendix-refrig-tie22}
\end{figure}

\begin{figure}[ht]
\centering
\begin{minipage}[t]{0.48\textwidth}
  \centering
  \includegraphics[width=\linewidth]{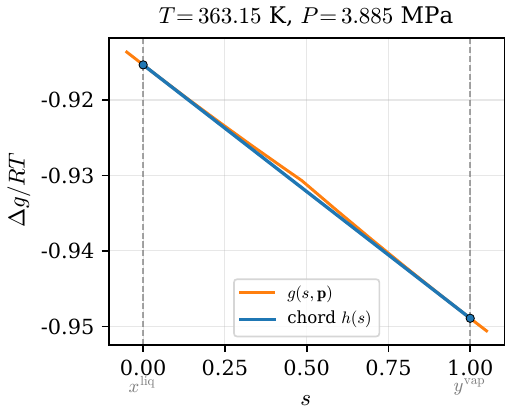}
\end{minipage}
\hfill
\begin{minipage}[t]{0.48\textwidth}
  \centering
  \includegraphics[width=\linewidth]{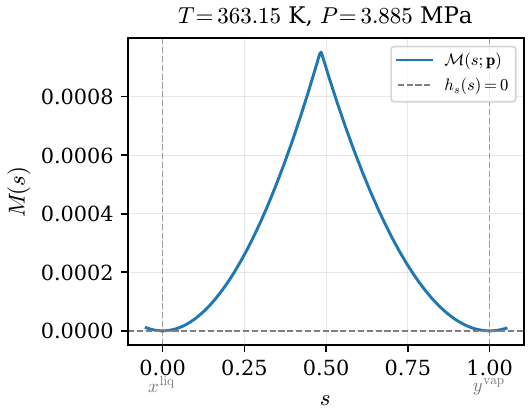}
\end{minipage}
\caption{Tie line 23 of the Kato--Nishiumi R-407C ternary set at $T = 363.15$~K, $P = 3.885$~MPa. Left: reduced Gibbs energy $g$ along the model tie-line section with the common-tangent chord $h$; right: dual manifold $\mathcal{M} = g - h$.}
\label{fig:appendix-refrig-tie23}
\end{figure}

\begin{figure}[ht]
\centering
\begin{minipage}[t]{0.48\textwidth}
  \centering
  \includegraphics[width=\linewidth]{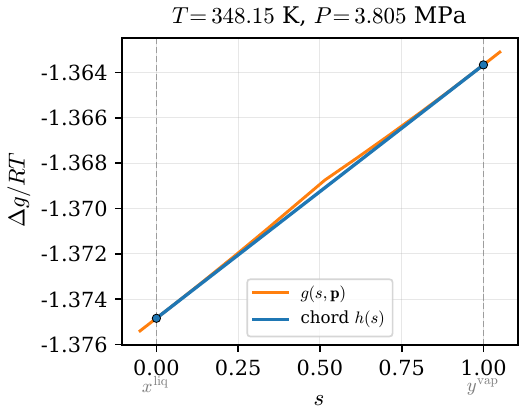}
\end{minipage}
\hfill
\begin{minipage}[t]{0.48\textwidth}
  \centering
  \includegraphics[width=\linewidth]{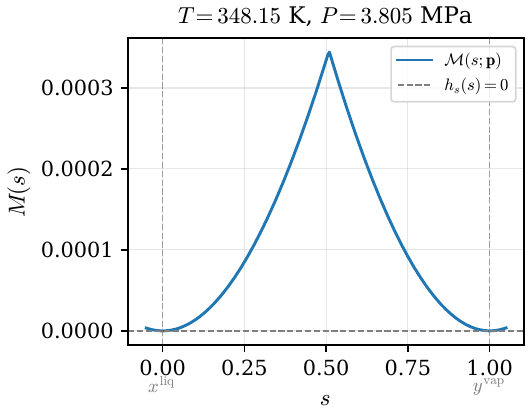}
\end{minipage}
\caption{Tie line 24 of the Kato--Nishiumi R-407C ternary set at $T = 348.15$~K, $P = 3.805$~MPa. Left: reduced Gibbs energy $g$ along the model tie-line section with the common-tangent chord $h$; right: dual manifold $\mathcal{M} = g - h$.}
\label{fig:appendix-refrig-tie24}
\end{figure}

\begin{figure}[ht]
\centering
\begin{minipage}[t]{0.48\textwidth}
  \centering
  \includegraphics[width=\linewidth]{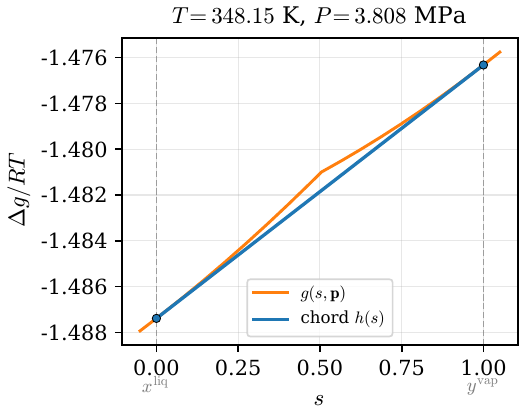}
\end{minipage}
\hfill
\begin{minipage}[t]{0.48\textwidth}
  \centering
  \includegraphics[width=\linewidth]{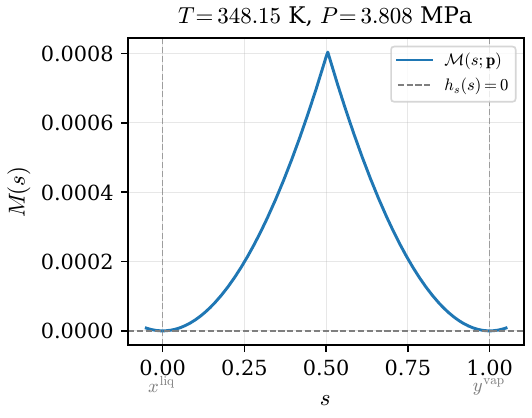}
\end{minipage}
\caption{Tie line 25 of the Kato--Nishiumi R-407C ternary set at $T = 348.15$~K, $P = 3.808$~MPa. Left: reduced Gibbs energy $g$ along the model tie-line section with the common-tangent chord $h$; right: dual manifold $\mathcal{M} = g - h$.}
\label{fig:appendix-refrig-tie25}
\end{figure}

\begin{figure}[ht]
\centering
\begin{minipage}[t]{0.48\textwidth}
  \centering
  \includegraphics[width=\linewidth]{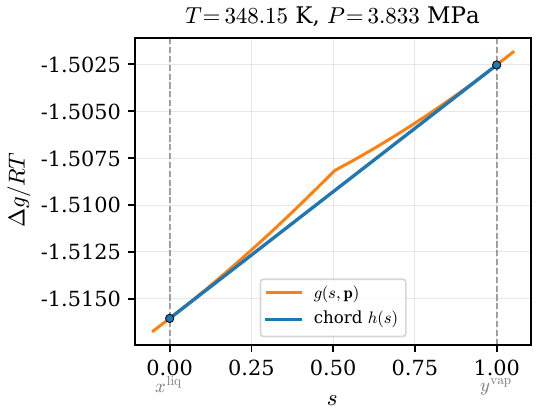}
\end{minipage}
\hfill
\begin{minipage}[t]{0.48\textwidth}
  \centering
  \includegraphics[width=\linewidth]{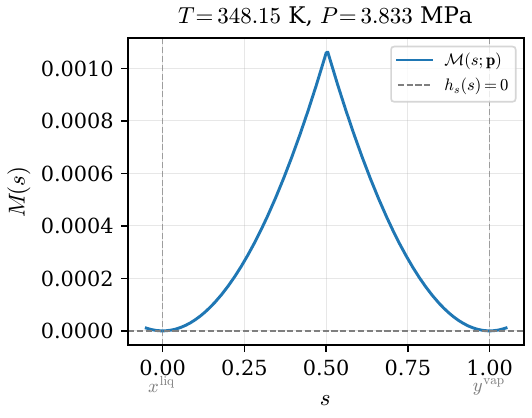}
\end{minipage}
\caption{Tie line 26 of the Kato--Nishiumi R-407C ternary set at $T = 348.15$~K, $P = 3.833$~MPa. Left: reduced Gibbs energy $g$ along the model tie-line section with the common-tangent chord $h$; right: dual manifold $\mathcal{M} = g - h$.}
\label{fig:appendix-refrig-tie26}
\end{figure}

\begin{figure}[ht]
\centering
\begin{minipage}[t]{0.48\textwidth}
  \centering
  \includegraphics[width=\linewidth]{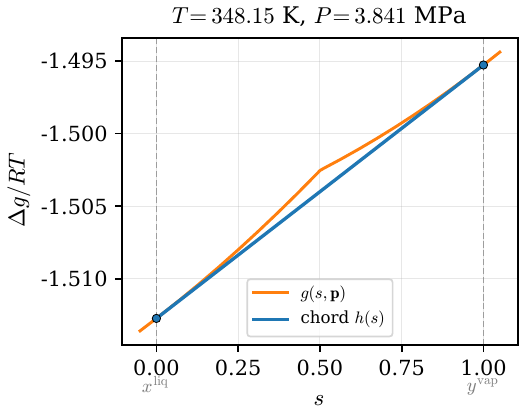}
\end{minipage}
\hfill
\begin{minipage}[t]{0.48\textwidth}
  \centering
  \includegraphics[width=\linewidth]{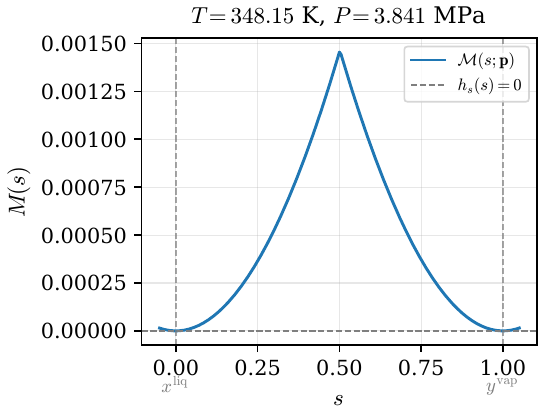}
\end{minipage}
\caption{Tie line 27 of the Kato--Nishiumi R-407C ternary set at $T = 348.15$~K, $P = 3.841$~MPa. Left: reduced Gibbs energy $g$ along the model tie-line section with the common-tangent chord $h$; right: dual manifold $\mathcal{M} = g - h$.}
\label{fig:appendix-refrig-tie27}
\end{figure}

\begin{figure}[ht]
\centering
\begin{minipage}[t]{0.48\textwidth}
  \centering
  \includegraphics[width=\linewidth]{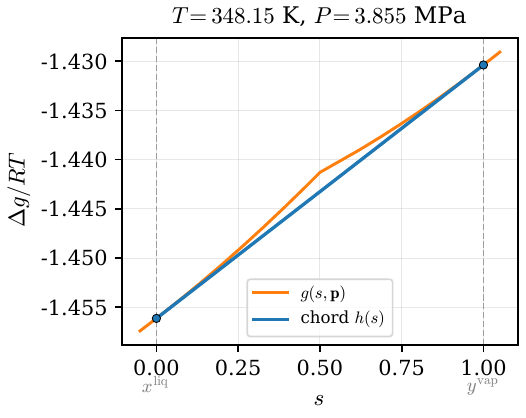}
\end{minipage}
\hfill
\begin{minipage}[t]{0.48\textwidth}
  \centering
  \includegraphics[width=\linewidth]{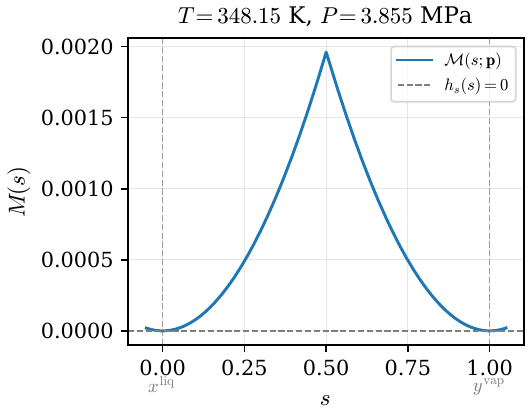}
\end{minipage}
\caption{Tie line 28 of the Kato--Nishiumi R-407C ternary set at $T = 348.15$~K, $P = 3.855$~MPa. Left: reduced Gibbs energy $g$ along the model tie-line section with the common-tangent chord $h$; right: dual manifold $\mathcal{M} = g - h$.}
\label{fig:appendix-refrig-tie28}
\end{figure}

\begin{figure}[ht]
\centering
\begin{minipage}[t]{0.48\textwidth}
  \centering
  \includegraphics[width=\linewidth]{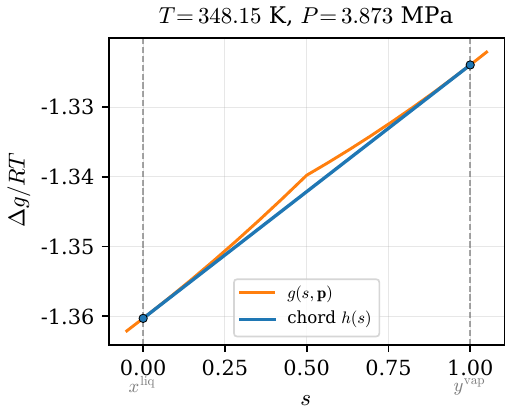}
\end{minipage}
\hfill
\begin{minipage}[t]{0.48\textwidth}
  \centering
  \includegraphics[width=\linewidth]{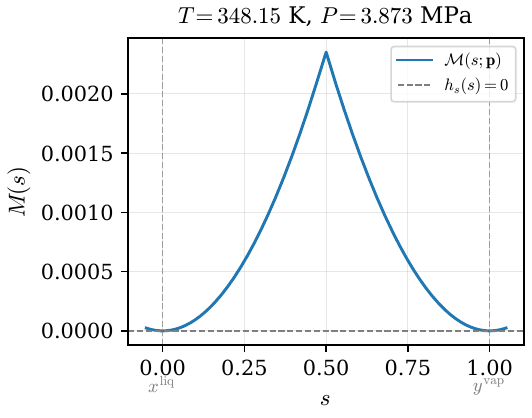}
\end{minipage}
\caption{Tie line 29 of the Kato--Nishiumi R-407C ternary set at $T = 348.15$~K, $P = 3.873$~MPa. Left: reduced Gibbs energy $g$ along the model tie-line section with the common-tangent chord $h$; right: dual manifold $\mathcal{M} = g - h$.}
\label{fig:appendix-refrig-tie29}
\end{figure}

\begin{figure}[ht]
\centering
\begin{minipage}[t]{0.48\textwidth}
  \centering
  \includegraphics[width=\linewidth]{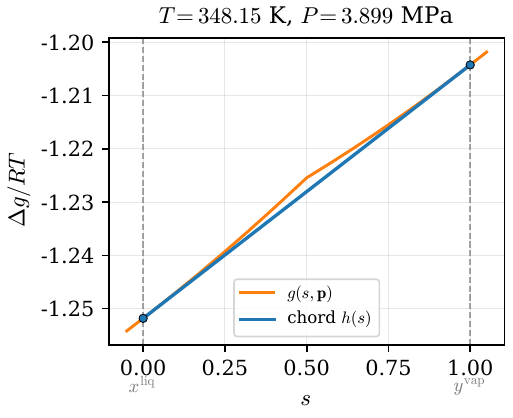}
\end{minipage}
\hfill
\begin{minipage}[t]{0.48\textwidth}
  \centering
  \includegraphics[width=\linewidth]{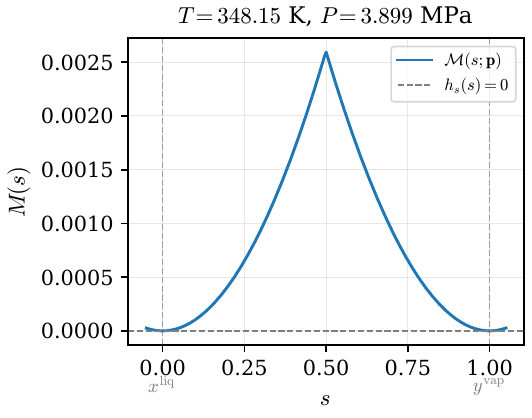}
\end{minipage}
\caption{Tie line 30 of the Kato--Nishiumi R-407C ternary set at $T = 348.15$~K, $P = 3.899$~MPa. Left: reduced Gibbs energy $g$ along the model tie-line section with the common-tangent chord $h$; right: dual manifold $\mathcal{M} = g - h$.}
\label{fig:appendix-refrig-tie30}
\end{figure}

\begin{figure}[ht]
\centering
\begin{minipage}[t]{0.48\textwidth}
  \centering
  \includegraphics[width=\linewidth]{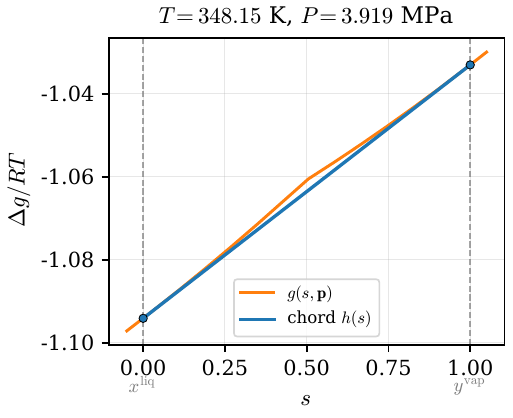}
\end{minipage}
\hfill
\begin{minipage}[t]{0.48\textwidth}
  \centering
  \includegraphics[width=\linewidth]{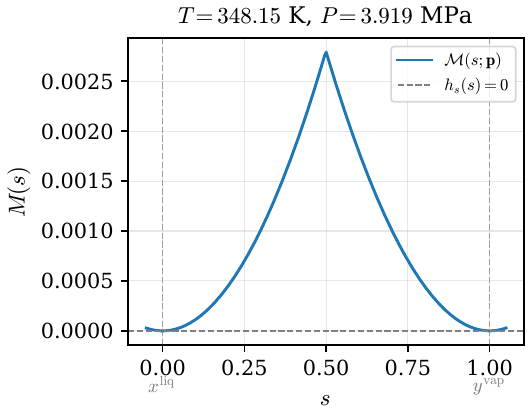}
\end{minipage}
\caption{Tie line 31 of the Kato--Nishiumi R-407C ternary set at $T = 348.15$~K, $P = 3.919$~MPa. Left: reduced Gibbs energy $g$ along the model tie-line section with the common-tangent chord $h$; right: dual manifold $\mathcal{M} = g - h$.}
\label{fig:appendix-refrig-tie31}
\end{figure}

\begin{figure}[ht]
\centering
\begin{minipage}[t]{0.48\textwidth}
  \centering
  \includegraphics[width=\linewidth]{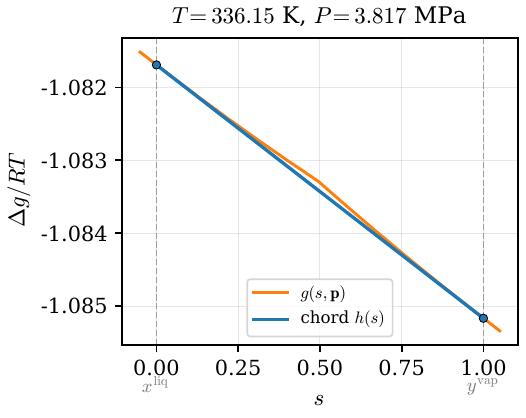}
\end{minipage}
\hfill
\begin{minipage}[t]{0.48\textwidth}
  \centering
  \includegraphics[width=\linewidth]{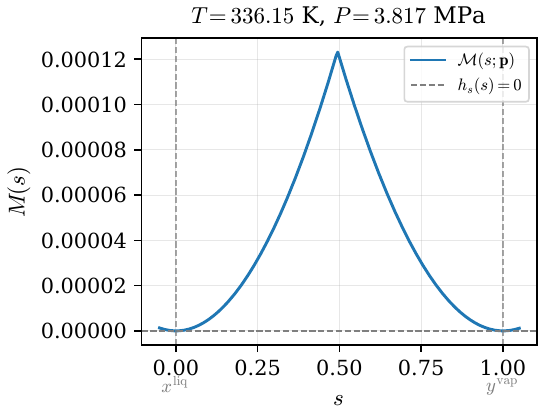}
\end{minipage}
\caption{Tie line 32 of the Kato--Nishiumi R-407C ternary set at $T = 336.15$~K, $P = 3.817$~MPa. Left: reduced Gibbs energy $g$ along the model tie-line section with the common-tangent chord $h$; right: dual manifold $\mathcal{M} = g - h$.}
\label{fig:appendix-refrig-tie32}
\end{figure}

\begin{figure}[ht]
\centering
\begin{minipage}[t]{0.48\textwidth}
  \centering
  \includegraphics[width=\linewidth]{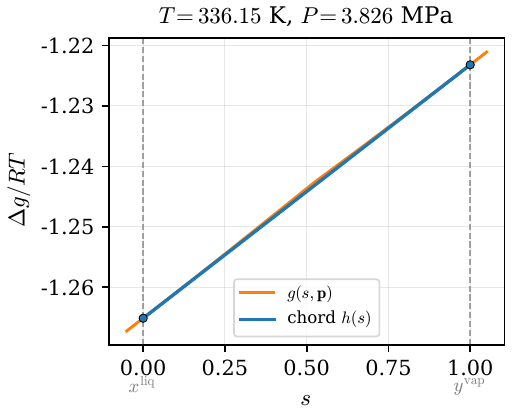}
\end{minipage}
\hfill
\begin{minipage}[t]{0.48\textwidth}
  \centering
  \includegraphics[width=\linewidth]{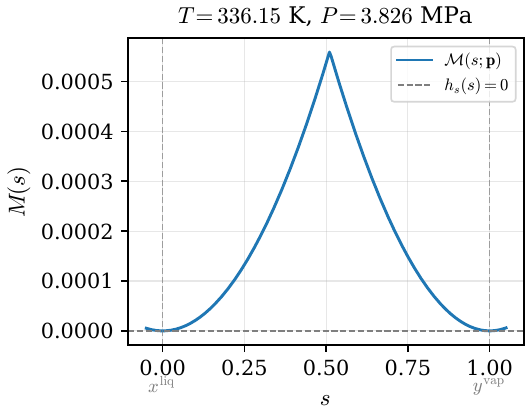}
\end{minipage}
\caption{Tie line 33 of the Kato--Nishiumi R-407C ternary set at $T = 336.15$~K, $P = 3.826$~MPa. Left: reduced Gibbs energy $g$ along the model tie-line section with the common-tangent chord $h$; right: dual manifold $\mathcal{M} = g - h$.}
\label{fig:appendix-refrig-tie33}
\end{figure}

\begin{figure}[ht]
\centering
\begin{minipage}[t]{0.48\textwidth}
  \centering
  \includegraphics[width=\linewidth]{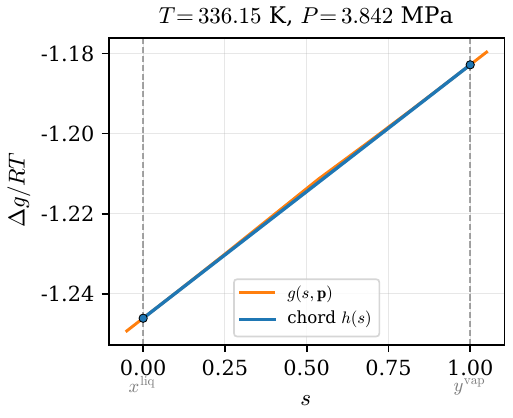}
\end{minipage}
\hfill
\begin{minipage}[t]{0.48\textwidth}
  \centering
  \includegraphics[width=\linewidth]{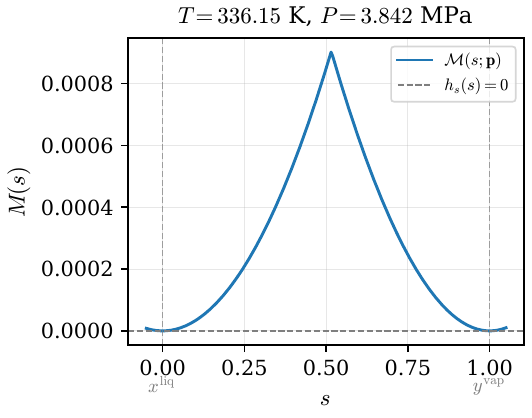}
\end{minipage}
\caption{Tie line 34 of the Kato--Nishiumi R-407C ternary set at $T = 336.15$~K, $P = 3.842$~MPa. Left: reduced Gibbs energy $g$ along the model tie-line section with the common-tangent chord $h$; right: dual manifold $\mathcal{M} = g - h$.}
\label{fig:appendix-refrig-tie34}
\end{figure}

\begin{figure}[ht]
\centering
\begin{minipage}[t]{0.48\textwidth}
  \centering
  \includegraphics[width=\linewidth]{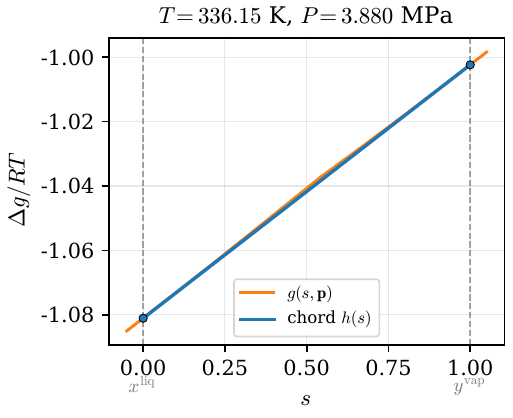}
\end{minipage}
\hfill
\begin{minipage}[t]{0.48\textwidth}
  \centering
  \includegraphics[width=\linewidth]{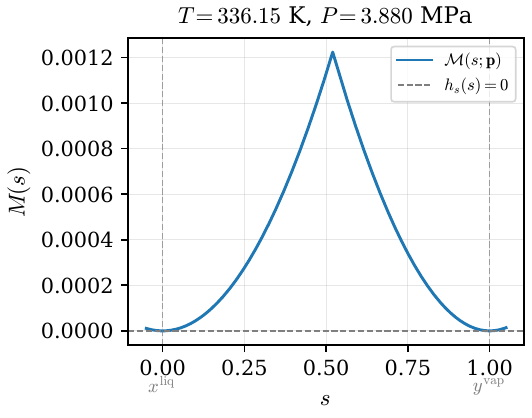}
\end{minipage}
\caption{Tie line 35 of the Kato--Nishiumi R-407C ternary set at $T = 336.15$~K, $P = 3.880$~MPa. Left: reduced Gibbs energy $g$ along the model tie-line section with the common-tangent chord $h$; right: dual manifold $\mathcal{M} = g - h$.}
\label{fig:appendix-refrig-tie35}
\end{figure}

\begin{figure}[ht]
\centering
\begin{minipage}[t]{0.48\textwidth}
  \centering
  \includegraphics[width=\linewidth]{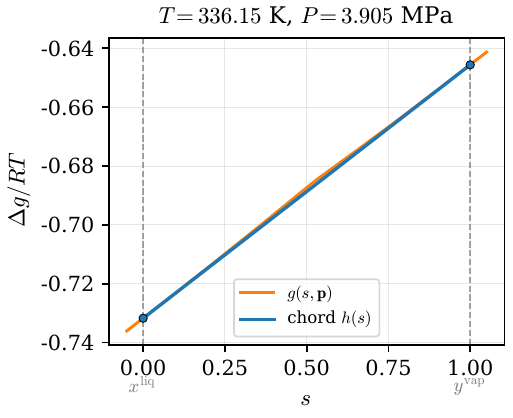}
\end{minipage}
\hfill
\begin{minipage}[t]{0.48\textwidth}
  \centering
  \includegraphics[width=\linewidth]{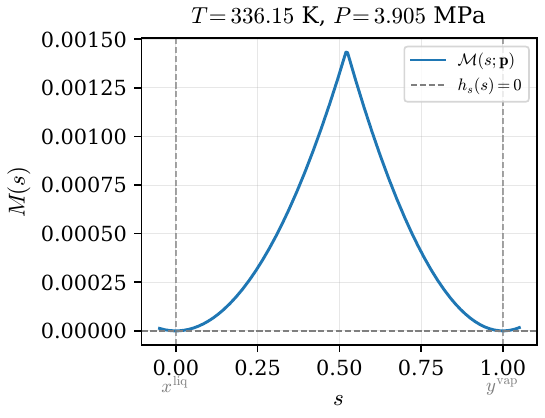}
\end{minipage}
\caption{Tie line 36 of the Kato--Nishiumi R-407C ternary set at $T = 336.15$~K, $P = 3.905$~MPa. Left: reduced Gibbs energy $g$ along the model tie-line section with the common-tangent chord $h$; right: dual manifold $\mathcal{M} = g - h$.}
\label{fig:appendix-refrig-tie36}
\end{figure}

\begin{figure}[ht]
\centering
\begin{minipage}[t]{0.48\textwidth}
  \centering
  \includegraphics[width=\linewidth]{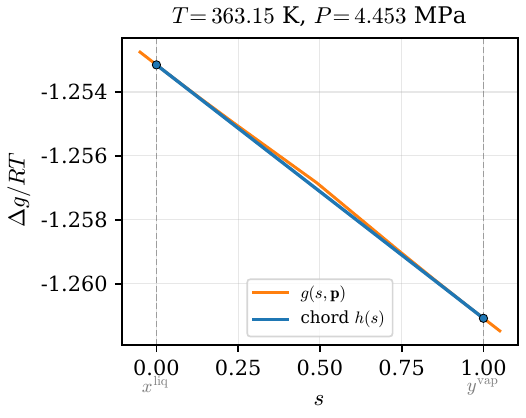}
\end{minipage}
\hfill
\begin{minipage}[t]{0.48\textwidth}
  \centering
  \includegraphics[width=\linewidth]{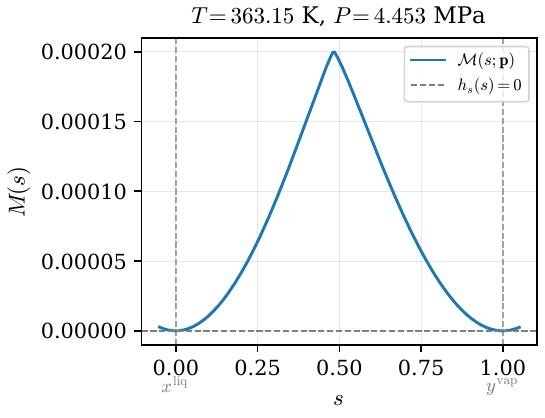}
\end{minipage}
\caption{Tie line 37 of the Kato--Nishiumi R-407C ternary set at $T = 363.15$~K, $P = 4.453$~MPa. Left: reduced Gibbs energy $g$ along the model tie-line section with the common-tangent chord $h$; right: dual manifold $\mathcal{M} = g - h$.}
\label{fig:appendix-refrig-tie37}
\end{figure}

\begin{figure}[ht]
\centering
\begin{minipage}[t]{0.48\textwidth}
  \centering
  \includegraphics[width=\linewidth]{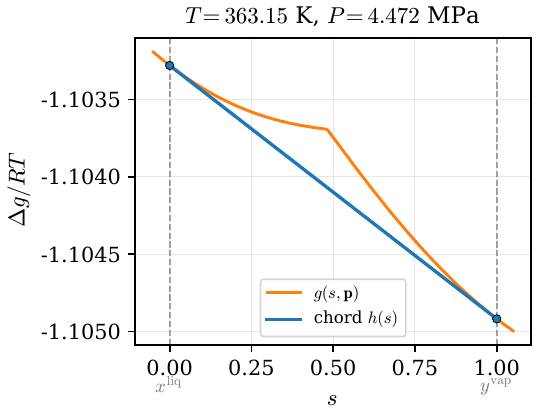}
\end{minipage}
\hfill
\begin{minipage}[t]{0.48\textwidth}
  \centering
  \includegraphics[width=\linewidth]{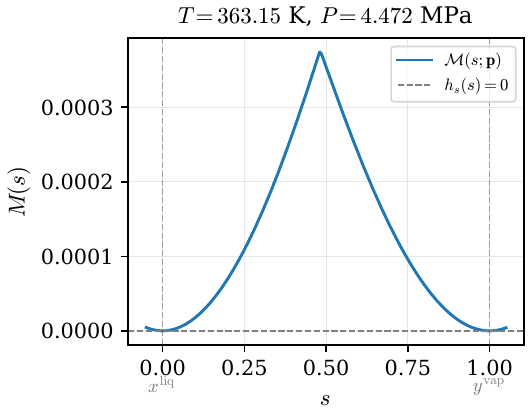}
\end{minipage}
\caption{Tie line 38 of the Kato--Nishiumi R-407C ternary set at $T = 363.15$~K, $P = 4.472$~MPa. Left: reduced Gibbs energy $g$ along the model tie-line section with the common-tangent chord $h$; right: dual manifold $\mathcal{M} = g - h$.}
\label{fig:appendix-refrig-tie38}
\end{figure}

\begin{figure}[ht]
\centering
\begin{minipage}[t]{0.48\textwidth}
  \centering
  \includegraphics[width=\linewidth]{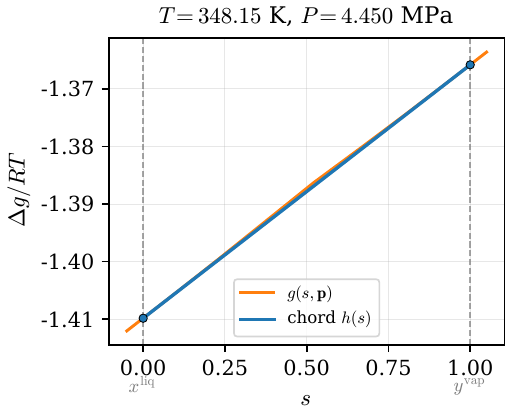}
\end{minipage}
\hfill
\begin{minipage}[t]{0.48\textwidth}
  \centering
  \includegraphics[width=\linewidth]{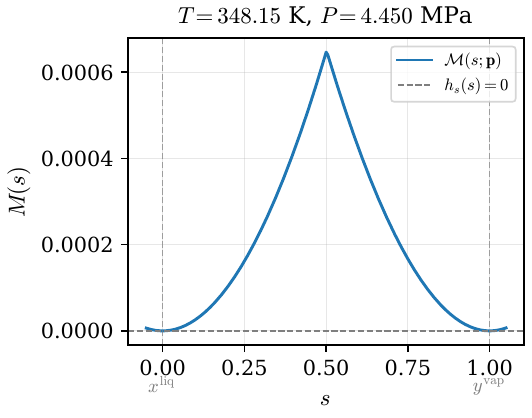}
\end{minipage}
\caption{Tie line 39 of the Kato--Nishiumi R-407C ternary set at $T = 348.15$~K, $P = 4.450$~MPa. Left: reduced Gibbs energy $g$ along the model tie-line section with the common-tangent chord $h$; right: dual manifold $\mathcal{M} = g - h$.}
\label{fig:appendix-refrig-tie39}
\end{figure}

\begin{figure}[ht]
\centering
\begin{minipage}[t]{0.48\textwidth}
  \centering
  \includegraphics[width=\linewidth]{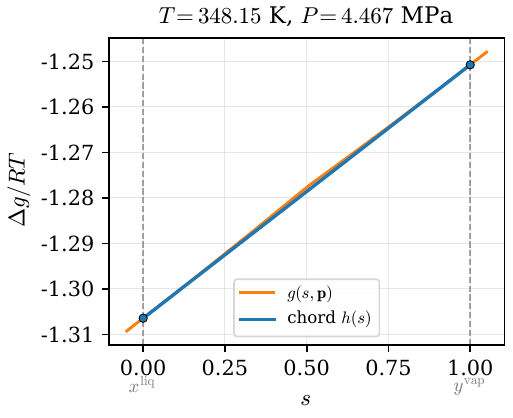}
\end{minipage}
\hfill
\begin{minipage}[t]{0.48\textwidth}
  \centering
  \includegraphics[width=\linewidth]{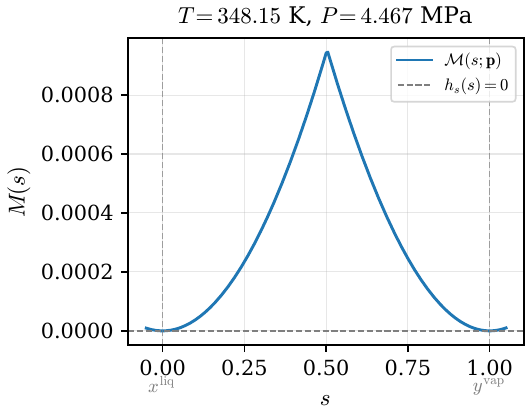}
\end{minipage}
\caption{Tie line 40 of the Kato--Nishiumi R-407C ternary set at $T = 348.15$~K, $P = 4.467$~MPa. Left: reduced Gibbs energy $g$ along the model tie-line section with the common-tangent chord $h$; right: dual manifold $\mathcal{M} = g - h$.}
\label{fig:appendix-refrig-tie40}
\end{figure}

\begin{figure}[ht]
\centering
\begin{minipage}[t]{0.48\textwidth}
  \centering
  \includegraphics[width=\linewidth]{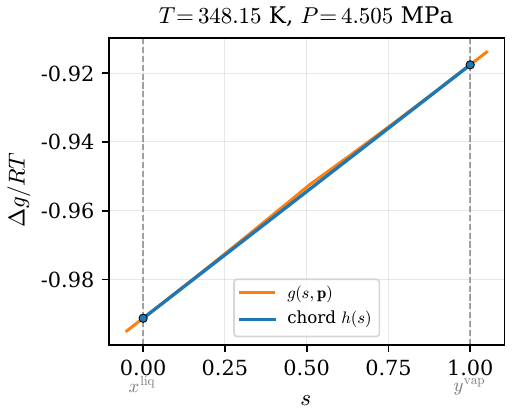}
\end{minipage}
\hfill
\begin{minipage}[t]{0.48\textwidth}
  \centering
  \includegraphics[width=\linewidth]{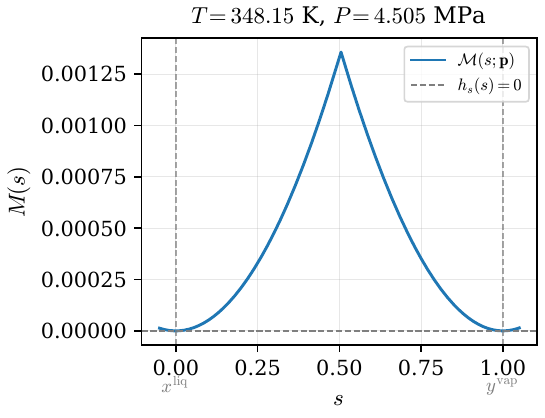}
\end{minipage}
\caption{Tie line 41 of the Kato--Nishiumi R-407C ternary set at $T = 348.15$~K, $P = 4.505$~MPa. Left: reduced Gibbs energy $g$ along the model tie-line section with the common-tangent chord $h$; right: dual manifold $\mathcal{M} = g - h$.}
\label{fig:appendix-refrig-tie41}
\end{figure}

\begin{figure}[ht]
\centering
\begin{minipage}[t]{0.48\textwidth}
  \centering
  \includegraphics[width=\linewidth]{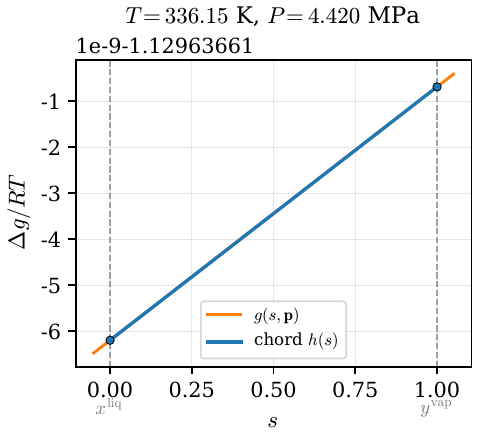}
\end{minipage}
\hfill
\begin{minipage}[t]{0.48\textwidth}
  \centering
  \includegraphics[width=\linewidth]{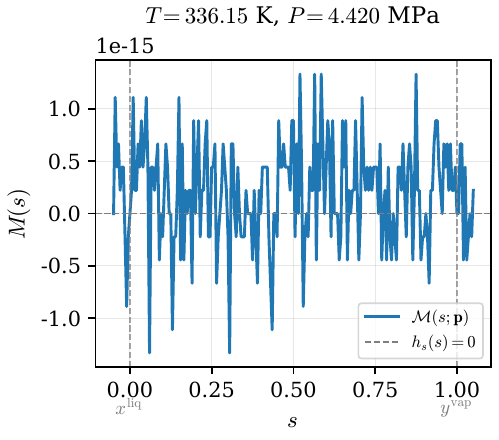}
\end{minipage}
\caption{Tie line 42 of the Kato--Nishiumi R-407C ternary set at $T = 336.15$~K, $P = 4.420$~MPa. Left: reduced Gibbs energy $g$ along the model tie-line section with the common-tangent chord $h$; right: dual manifold $\mathcal{M} = g - h$.}
\label{fig:appendix-refrig-tie42}
\end{figure}

\begin{figure}[ht]
\centering
\begin{minipage}[t]{0.48\textwidth}
  \centering
  \includegraphics[width=\linewidth]{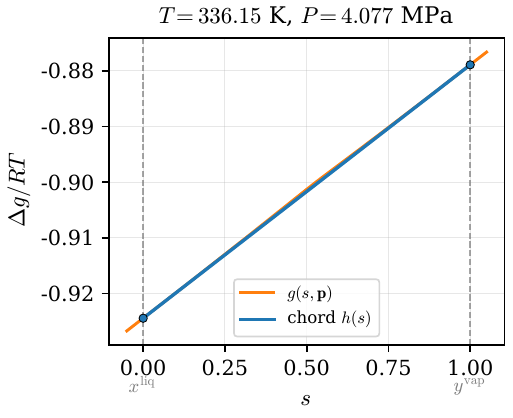}
\end{minipage}
\hfill
\begin{minipage}[t]{0.48\textwidth}
  \centering
  \includegraphics[width=\linewidth]{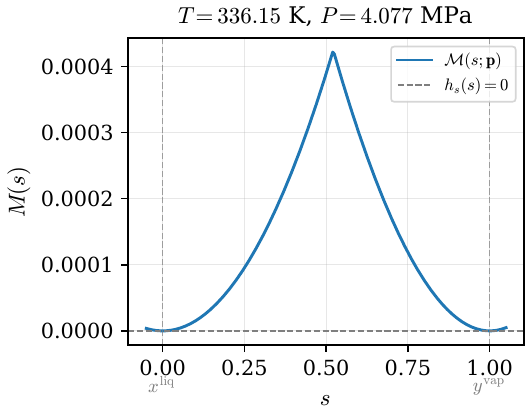}
\end{minipage}
\caption{Tie line 43 of the Kato--Nishiumi R-407C ternary set at $T = 336.15$~K, $P = 4.077$~MPa. Left: reduced Gibbs energy $g$ along the model tie-line section with the common-tangent chord $h$; right: dual manifold $\mathcal{M} = g - h$.}
\label{fig:appendix-refrig-tie43}
\end{figure}

\begin{figure}[ht]
\centering
\begin{minipage}[t]{0.48\textwidth}
  \centering
  \includegraphics[width=\linewidth]{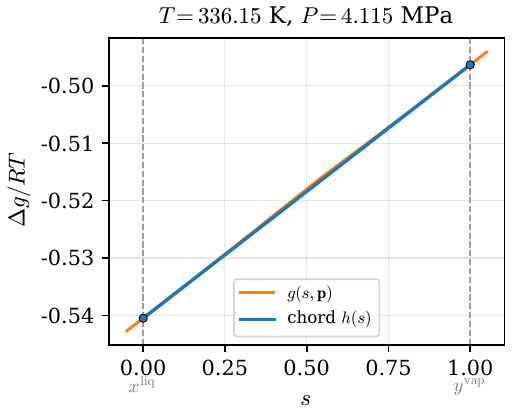}
\end{minipage}
\hfill
\begin{minipage}[t]{0.48\textwidth}
  \centering
  \includegraphics[width=\linewidth]{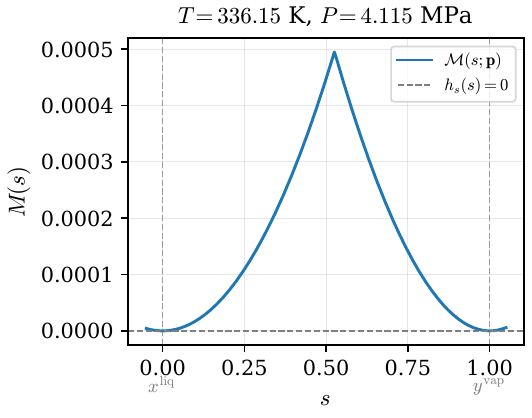}
\end{minipage}
\caption{Tie line 44 of the Kato--Nishiumi R-407C ternary set at $T = 336.15$~K, $P = 4.115$~MPa. Left: reduced Gibbs energy $g$ along the model tie-line section with the common-tangent chord $h$; right: dual manifold $\mathcal{M} = g - h$.}
\label{fig:appendix-refrig-tie44}
\end{figure}
