# Supplementary material for: A geometric reformulation of the bilevel parameter optimization problem to a single level non-linear programming problem with applications to phase equilibria
Source: arXiv:2608.17806 source file (2026-08-18)
Supplement: Supplementary file 4 [file supp_ccs_refrig_per_point.tex]

% !TEX root = ../supplementary_S3_ccs_refrig.tex
% ------------------------------------------------------------------
% Supplementary Material S3 body: per-tie-line Gibbs / dual-manifold
% archives for the CCS quaternary and refrigerant R-407C cases (main
% manuscript, CCS and refrigerant results sections). Figure blocks are
% generated by the plot.py of figures/appendix-ccs-ternary/ and
% figures/appendix-refrig-ternary/ from raw data produced by
% scripts_ccs_manuscript_figdata.py / scripts_refrig_manuscript_figdata.py
% at the fitted parameters.
% ------------------------------------------------------------------

Analogously to the sour-gas archive of Supplementary Material~S2,
this supplement records the
reduced Gibbs energy and dual manifold along every model tie-line
section of the two remaining industrial validation sets, evaluated at
the respective fitted parameters $\mathbf{p}^{\star}$ with the section
construction defined there. Both records are fully defect-free:
$\mathcal{M} \geq 0$ holds along every section with equality only at
the two phase compositions.

\subsection{CCS quaternary: CO$_2$/Ar/O$_2$ validation tie lines}
\label{supp:ccs-per-point}

The 18 ternary validation tie lines
of~\cite{CoqueletArpentinier2014} at the CO$_2$-$X$ parameters
reported in the CCS results section of the main manuscript, with air
pairs ideal ($k_{a,ij}=0$).

\input{figures/appendix-ccs-ternary/appendix-ccs-ternary_figure_blocks}

\clearpage
\subsection{Refrigerant R-407C: ternary validation tie lines}
\label{supp:refrig-per-point}

The 44 ternary validation tie lines of~\cite{KatoNishiumi2006} at
the binary-fitted parameters reported in the refrigerant results
section of the main manuscript.

\input{figures/appendix-refrig-ternary/appendix-refrig-ternary_figure_blocks}
