# Supplementary material for: A geometric reformulation of the bilevel parameter optimization problem to a single level non-linear programming problem with applications to phase equilibria
Source: arXiv:2608.17806 source file (2026-08-18)
Supplement: Supplementary file 5 [file supp_sour_gas_per_point.tex]

% !TEX root = ../supplementary_S2_sour_gas.tex
% ------------------------------------------------------------------
% Supplementary Material S2 body: per-tie-line Gibbs / dual-manifold
% archive for the sour-gas ternary case (main manuscript, sour-gas
% results section). The 31 figure blocks are generated by
% figures/appendix-sour-gas-ternary/plot.py (which also emits
% figure_blocks.tex) from raw data produced by
% scripts_sour_gas_manuscript_figdata.py at the fitted parameters.
% ------------------------------------------------------------------

In this supplement we archive, for every one of the 31 experimental
ternary tie lines of Theveneau et al.~\cite{Theveneau2020}
% [PDF: page 3, Table 2 and page 4, Table 3] - the 31 validation tie lines
used to validate the sour-gas case of the main manuscript,
the reduced Gibbs energy and the dual manifold evaluated at the fitted
parameters $\mathbf{p}^{\star}$. Because the equilibrium here is
vapor--liquid at elevated pressure, the one-dimensional section shown
for each tie line is taken along the \emph{model} tie line: the
segment $\mathbf{x}(s) = (1-s)\,\mathbf{x}^{\mathrm{exp}}_{\mathrm{I}}
+ s\,\mathbf{y}^{\mathrm{mod}}$, $s \in [-0.05, 1.05]$, joining the
experimental liquid composition to the vapor composition returned by
the bubble-point calculation at $(T_i, p^{\mathrm{mod}}_i)$. For each
tie line the left panel shows the minimum-root reduced Gibbs energy
$g(\mathbf{x}(s), \mathbf{p}^{\star})$ together with the
common-tangent chord $h$ between the two phase compositions; the
right panel shows the dual manifold
$\mathcal{M}(\mathbf{x}(s); \mathbf{p}^{\star}) = g - h$, whose
negative part $[\mathcal{M}]_{-}$ enters the bilevel objective. A
defect-free solution requires $\mathcal{M} \geq 0$ along the entire
section, with equality only at the two phase compositions. The plots
below constitute the point-by-point record of that property for the
regressed sour-gas parameters: 27 of the 31 sections are defect-free
to numerical tolerance, while the four highest-pressure near-critical
tie lines (18, 19, 24 and 27; $p = 13.6$--$15.4$~MPa) show shallow
negative lobes of magnitude
$\lvert \min \mathcal{M} \rvert \leq 2.5 \times 10^{-5}$, visible in
the corresponding manifold panels and discussed in the sour-gas
results section of the main manuscript.

\input{figures/appendix-sour-gas-ternary/appendix-sour-gas-ternary_figure_blocks}
