# Supplementary material for: A geometric reformulation of the bilevel parameter optimization problem to a single level non-linear programming problem with applications to phase equilibria
Source: arXiv:2608.17806 source file (2026-08-18)
Supplement: Supplementary file 8 [file supplementary_S3_ccs_refrig.tex]

%%
%% Supplementary Material S3 to:
%% A geometric reformulation of the bilevel parameter optimization problem
%% to a single level non-linear programming problem with applications to
%% phase equilibria.
%%
%% Per-tie-line Gibbs and dual-manifold plots for the CCS and
%% refrigerant validation cases. Body lives in
%% sections/supp_ccs_refrig_per_point.tex.
%% Build: latexmk -pdf supplementary_S3_ccs_refrig.tex

\documentclass[preprint,12pt, a4paper]{elsarticle}

\usepackage{graphicx}
% The per-tie-line archives queue up ~120 consecutive figure floats;
% enlarge the float register pool so LaTeX can hold them until each
% page flushes.
\extrafloats{200}

% Math
\usepackage{amsmath}
\usepackage{amsfonts}
\usepackage{amssymb}
\usepackage{mathtools}

% References
\usepackage[plainpages=false, pdfpagelabels]{hyperref}
\usepackage{cleveref}% Has to be loaded after hyperref

% Supplementary numbering: S3.x
\renewcommand{\thesection}{S3.\arabic{section}}
\renewcommand{\thefigure}{S3.\arabic{figure}}
\renewcommand{\thetable}{S3.\arabic{table}}
\renewcommand{\theequation}{S3.\arabic{equation}}

\begin{document}

\begin{frontmatter}
\title{Supplementary Material S3: Per-tie-line Gibbs and dual-manifold
plots for the CCS and refrigerant validation cases\\[1ex]
\normalsize{Supplement to: A geometric reformulation of the bilevel
parameter optimization problem to a single level non-linear programming
problem with applications to phase equilibria}}
\end{frontmatter}

\section{Per-tie-line Gibbs and dual-manifold plots for the CCS and refrigerant cases}
\label{supp:ccs-refrig-per-point}
\input{sections/supp_ccs_refrig_per_point}

\bibliographystyle{elsarticle-num}
\bibliography{references}

\end{document}
